# Supplementary material for: Learning To Cut By Looking Ahead: Cutting Plane Selection via Imitation Learning
Source: arXiv:2206.13414 source file (2022-06-27)
Supplement: Supplementary file 4 [file dump.tex]

%%%%%%%%%%%%%%%%%%%%%%%%% DUMPING GROUND %%%%%%%%%%%%%%%%%%%%%%%%% 
\iffalse
\section{\red{[dump from main paper / old versions]}}

\subsection{Custom Selection Procedure}

\blue{[We don't use this setup for all experiments, so tune the section accordingly].
Distinction between single and multi should come later on ML. multi cuts added from the same pool. Method part only: selecting cut from a pool, scip is also iterative! scores are computed at the beginning, cuts are sorted by score, select best cut and keep track of it, filter n-1 cuts to remove the too parallel ones, of the remaining, select best cut still based on the initial score. Phrase cut selection problem: given pool, select one and apply it. The rest are other decisions (if to select, when to do separation, etc)(write in conclusions), relevant for selection, e.g., in nn verification. KEEP IT SIMPLE: PROBLEM IS WHICH CUT TO SELECT. 

} 
Because combining several (and diverse) cuts in each round yields tighter formulations, we allow the expert to select multiple cuts per round, in a sequential manner. 
Specifically, we select the cuts that make up $S^k$ one by one, clearing the cutpool to mark the end of a round. This way, we only need a single-cut selector iteratively applied to a fixed cutpool to select multiple cuts per round, thus avoiding to frame the selection problem on subsets of $\mathscr{C}^k$. 
Algorithm~\ref{alg:multicut} describes our procedure, specified by a triple (\textit{scorer}, \textit{stopper}, \textit{filter}) where
\begin{itemize}
    \item \textit{scorer} defines the criterion according to which a cut should be scored and accordingly selected from the current cutpool (e.g., lookahead, efficacy, expected improvement); 
    % \footnote{Ties can be broken, e.g., lexicographically on the cuts' names.} 
    \item \textit{stopper} prescribes when the separation procedure should be halted (e.g., due to stalling or reaching of an iteration limit), and the cutpool cleared;
    \item \textit{filter} specifies how the cutpool should be filtered after the selection of a cut (e.g., to avoid parallelism in $S^k$).
\end{itemize}
A single-cut algorithm is easily obtained by setting an appropriate \textit{stopper} criterion.\footnote{The $\mathit{maxcuts}$ parameter in Algorithm~\ref{alg:multicut} functions as and takes its value from the \texttt{separating/maxcutsroot} parameter in SCIP (2000 at default).}
Note that after a cut is selected it is added to the LP relaxation; the next cut will then be picked from a filtered cutpool, based on scores which have been recomputed on the updated relaxation. 
Updating scores dynamically (within the round) differentiates our procedure from the SCIP one, which is instead equivalent to selecting score-maximizing cuts one by one, only based on beginning-of-the-round scores. 
% a predetermined number of top-ranked cuts are selected simultaneously from the available ones


\begin{algorithm}[t]
\caption{Multi-cut selection procedure (round $k+1$)}\label{alg:multicut}
\begin{algorithmic}
  \STATE {\bfseries Input:} Solved relaxation $P^{k}$, cutpool $\mathscr{C}^{k+1}$, $\mathit{maxcuts}$ parameter. Functions (\textit{scorer}, \textit{stopper}, \textit{filter}).
  \STATE {\bfseries Output:} Selected cuts $S^{k+1}\subseteq\mathscr{C}^{k+1}$ defining $P^{k+1}$.
  \STATE $S^{k+1}\coloneqq\emptyset$
  \STATE $P^{k+1}\coloneqq P^k$ %\hfill\COMMENT{The relaxation solved in this round}
  \WHILE{$\mathscr{C}^{k+1}\neq\emptyset$ and $|S^{k+1}|<\mathit{maxcuts}$}
    \STATE $C_{j^*} = \argmax_{C_j \in\mathscr{C}^{k+1}} {\mathit{scorer}(C_j, P^{k+1})}$ %\hfill\COMMENT{Determine best cut with LA scores on $P^{k+1}$}
    \IF{$\mathit{stopper}(C_{j^*})$}
    \STATE {\bfseries break} %\hfill\COMMENT{Stop if the cut should not be added}
    \ELSE
    \STATE $S^{k+1}\gets S^{k+1}\cup\{C_{j^*}\}$
    \STATE $P^{k+1}\gets P^{k+1}\cap\{\pi^Tx \le\pi_0\}$ %\hfill\COMMENT{Add cut $C_{j^*}$ to $P^{k+1}$}
    \STATE $\mathscr{C}^{k+1}\gets \mathscr{C}^{k+1}\setminus\{C_{j^*}\}$
    \STATE $\mathscr{C}^{k+1}\gets\mathit{filter}(\mathscr{C}^{k+1})$ %\hfill\COMMENT{Filter the cutpool now that $C_{j^*}$ was selected}
    \ENDIF
  \ENDWHILE
  \STATE {\bfseries return} $S^{k+1}$
\end{algorithmic}
\end{algorithm}

\paragraph{Lookahead Expert Design}{
We implement the selection procedure of Algorithm~\ref{alg:multicut} in a customized SCIP version. 
Our interface with the solver covers ten different separators, namely, \texttt{aggregation}, \texttt{clique}, \texttt{disjunctive}, \texttt{flowcover}, \texttt{gomory}, \texttt{impliedbounds}, \texttt{mcf}, \texttt{oddcycle}, \texttt{strongcg}, \texttt{zerohalf}. 
% we given more details in \blue{Appendix~\ref{app:scip}}. 

The LA cut selector is obtained by using LA scores \eqref{eq:lascore} as the \textit{scorer} function. Operationally, at a given round $k+1$ with LP relaxation defined by $P^{k}$, all candidate cuts in $\mathscr{C}^{k+1}$ are tested one by one (setting SCIP in diving mode) and their bound improvements are registered as LA scores $s_\textsc{la}$, which are used to iteratively identify $S^{k+1}\subseteq\mathscr{C}^{k+1}$. Plugging-in different \textit{scorer} heuristics allows to compare cut selection criteria; 
the \textit{scorer} used in SCIP default is a weighted sum of objective parallelism, integer support and efficacy scores (see Table~\ref{tab:baselines}).
% (Lookahead, SCIPCutBudget, ParallelismSCIP)
% (SCIPScore, ..., ParallelismSCIP)

Our \textit{stopper} criterion is based on the notion of ``cut budget'' used by SCIP: for each instance, we retrieve the average number of cuts applied in each round by SCIP default separators and selectors. We then enforce this budget as an instance-specific limit to the cuts added in each of our rounds. This ensures a fairer and easier comparison of bound improvements with the SCIP selection process, whose stopping criterion is more complex and procedural, and based on multiple tuned parameters. 
Finally, our LA expert employs a \textit{filter} mechanism based on parallelism that mimics the one in SCIP, maintaining in the cutpool only cuts which are ``good'' and are not too parallel with the already selected $C_{j^*}$.\footnote{Similarly to SCIP's own filtering procedure, a ``good'' cut is determined within a factor \texttt{separating/goodscorefac} of the maximum SCIP score; we also use SCIProwGetParallelism and parameters \texttt{separating/goodmaxparallroot}, \texttt{separating/maxparallroot}.}
}


% \paragraph{Baselines and Evaluation}{
% \blue{
% [This paragraph could also be spread throughout different sections, introducing things when they are first used.]
% \begin{itemize}
%     \item Say what are the score-based rules that we include in our plots. Explain the Scikit-learn baseline. 
% \end{itemize}
% }

% We use IGC to compare our expert to other score-based baselines. 
% The metric makes use of the optimal value $z^{\mathit{OPT}}$ for each problem, which we compute beforehand using SCIP at default mode; we do not use knowledge of $z^{\mathit{OPT}}$ or IGC to inform the LA expert. \blue{Another thing we compute beforehand is SCIP cut budget.} 
% \blue{
% \begin{itemize}
%     \item Introduce ``regret'' and ``dual integrality integral'' metrics for test. 
% \end{itemize}
% }
% }

% \paragraph{Setup}{
% \blue{
% \begin{itemize}
%     \item SCIP parametric setting (no primal heuristics, presolve on, override of SCIP separation with node limit, minefficacyroot and random branching), specs for our separators (this could also be mentioned before in data collection). 
%     \item ML setup (optimizer, hyper-parameters, etc.). Leave hardware specs for Appendix.
% \end{itemize}
% }
% }

% The LA expert selects cuts by explicitly optimizing the dual bound improvement. We ask whether maximizing the bound improvement at the root node produces an advantage in later optimization stages, beyond the root node. In other words, is following the LA criterion beneficial for solving a MILP to proven optimality, with procedures like Branch and Cut (B\&C) or B\&B? 
% We run controlled experiments to compare the optimization performance of SCIP on a given model, with or without LA cut separation enabled. In particular, we run \blue{XXX} rounds of multi-cut LA separation at the root node, before resetting the solver to its default behavior to complete the MILP optimization. We compare the SCIP outcomes on these models to the performance attained without our cutloop, when the optimization is continued \emph{(i)} at SCIP default setting (potentially applying its own cutting planes at subsequent nodes of the B\&C tree), and \emph{(ii)} in `no separation' setting, i.e., running the default SCIP B\&B without additional cutting planes. The metrics we rely on for this evaluation are the total number of nodes explored in the search tree (nnodes), the total number of LP iteration solved (nlpiters) and runtimes. Results are summarized in Figure/Table \ref{fig:multi-igc-bb}. 

% \begin{figure*}[tb]
%   \dummyfig{Plot IGC after multiple rounds at the root node, for various baselines and the learned multi-cut LA rule. Use Ecole datasets (4, of which size?). Possibly include more than one ML model.}
%   \hfill
%   \dummyfig{Compare SCIP performance w/ and w/o LA cut selection at the root node: barplots of nodes, runtimes, iterations (and/or extensive Table in appendix). Use Ecole datasets (4, of which size?). Possibly include more than one ML model.}
%   \caption{Multi-cut trained rules compared to other baseline scores, and effect on B\&C optimization, on Ecole instances.}
%   \label{fig:multi-igc-bb}
% \end{figure*}
\fi


%%%%%%%%%%%%%%%%%%%%%%%%%%%%%%%%%%%%%%%%%%%%%%%%%%%%%%%%%%%%%%%%%%%%%%%%%%%%%%%
%%%%%%%%%%%%%%%%%%%%%%%%%%%%%%%%%%%%%%%%%%%%%%%%%%%%%%%%%%%%%%%%%%%%%%%%%%%%%%%
